# Supplementary material for: Learning Representations by Maximizing Mutual Information Across Views
Source: arXiv:1906.00910 source file (2019-07-08)
Supplement: Supplementary file 2 [file SEC_appendix.tex]

\begin{figure*}[ht]
    \centering
    \includegraphics[scale=0.1035]{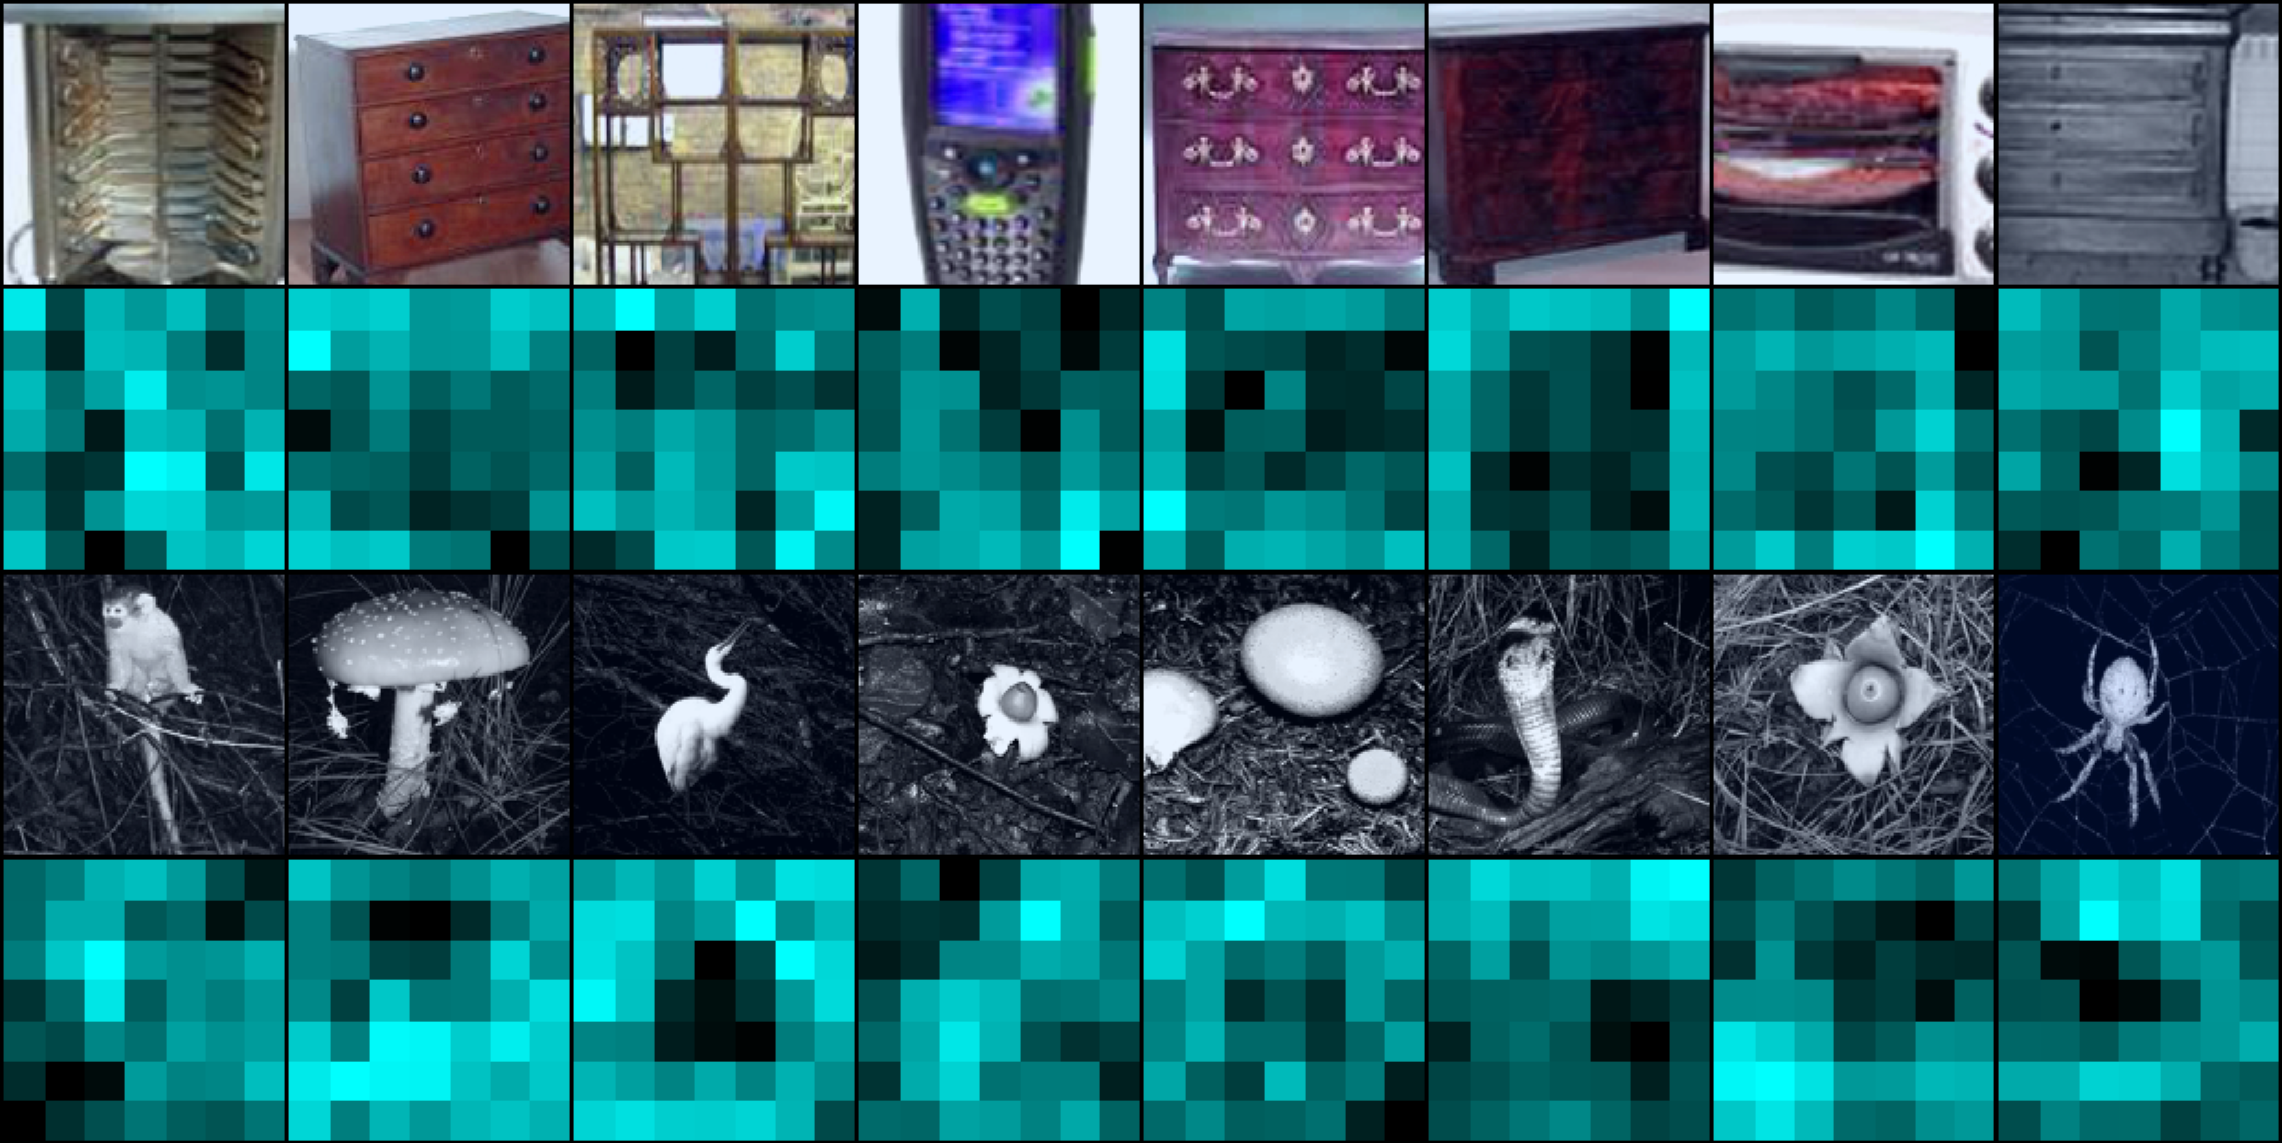}
    \includegraphics[scale=0.0985]{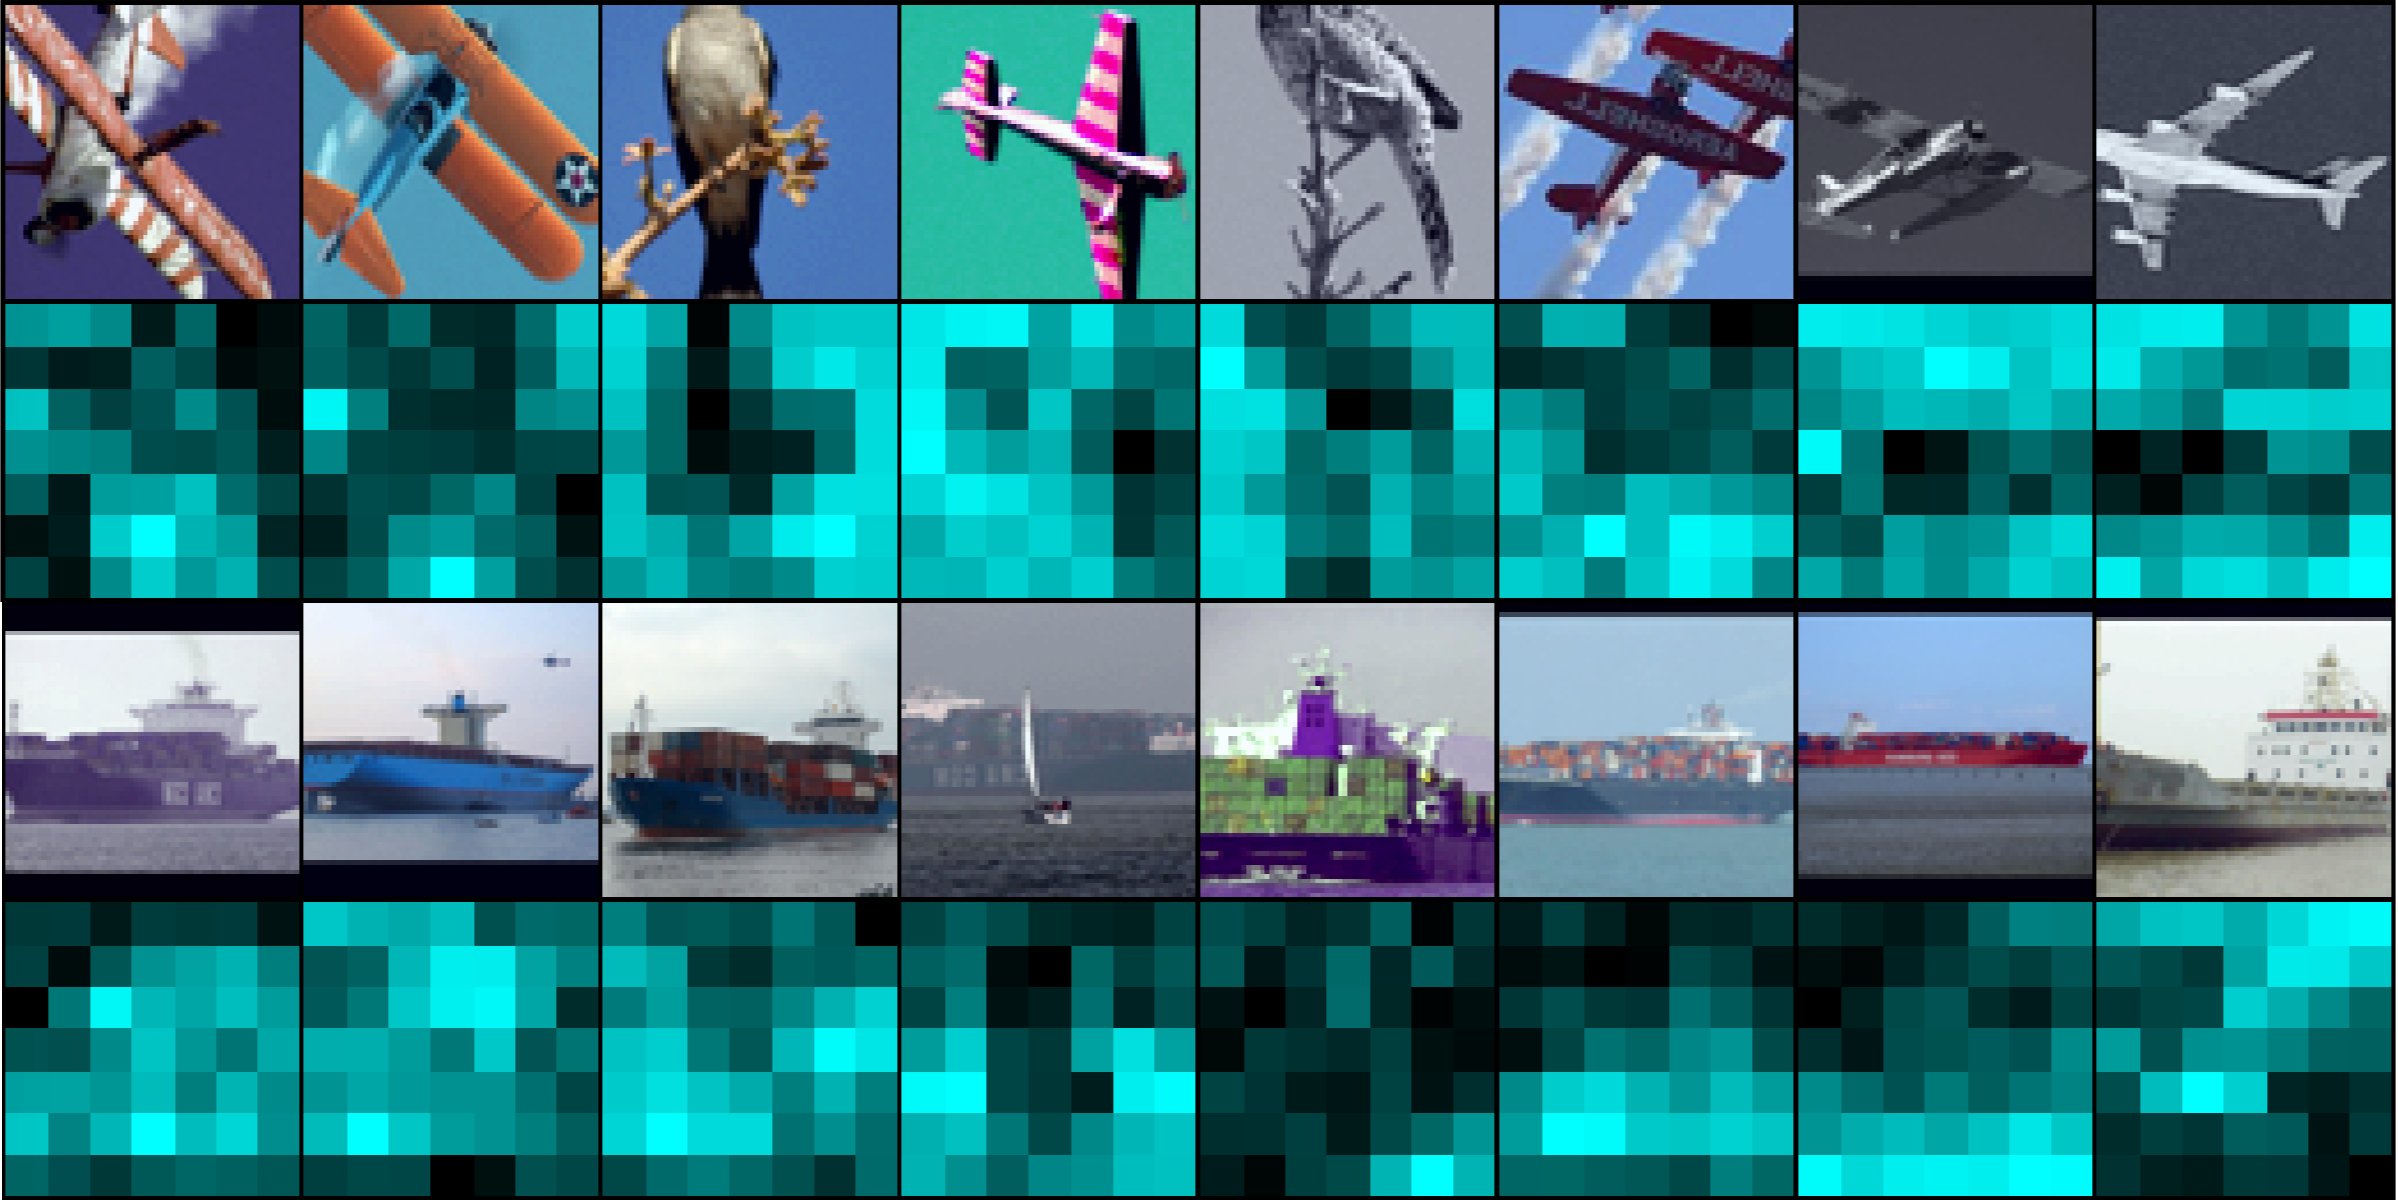}
    \caption{Common failure modes on ImageNet and STL10. The left group of images is from ImageNet and the right group is from STL10. The left-most image in the top row of each row pair is the query image and the next seven images are the seven nearest neighbors according to cosine similarity between global features $f_1(x)$. On ImageNet we retrieved from a buffer holding roughly 25\% of the training set, and on STL10 we retrieved from the whole training set. The second row in each row pair shows the similarity score $\phi_1(f_1(x))^{\top} \phi_7(f_7(x^{\prime}))$ between the global features of the query image $x$ and the features from the $7 \times 7$ feature layer for each retrieved image $x^{\prime}$. The top two rows for ImageNet exhibit a pattern where global similarity is skewed by the presence of compression artifacts, which affect all image patches. The bottom images for ImageNet and top images for STL10 show a common pattern where similarity between global features seems to be dominated by similarity of background patches, which are more numerous and more homogeneous than foreground patches. The bottom STL10 images show an interesting result where, in the fourth column, the foreground object does not match the query image but the background object does. And, this is visible in the similarity scores. These examples present clear motivation for future work.}
    \label{fig:model_failure}
    \vspace{-0.5cm}
\end{figure*}

\begin{figure}
    \centering
    \includegraphics[scale=0.0985]{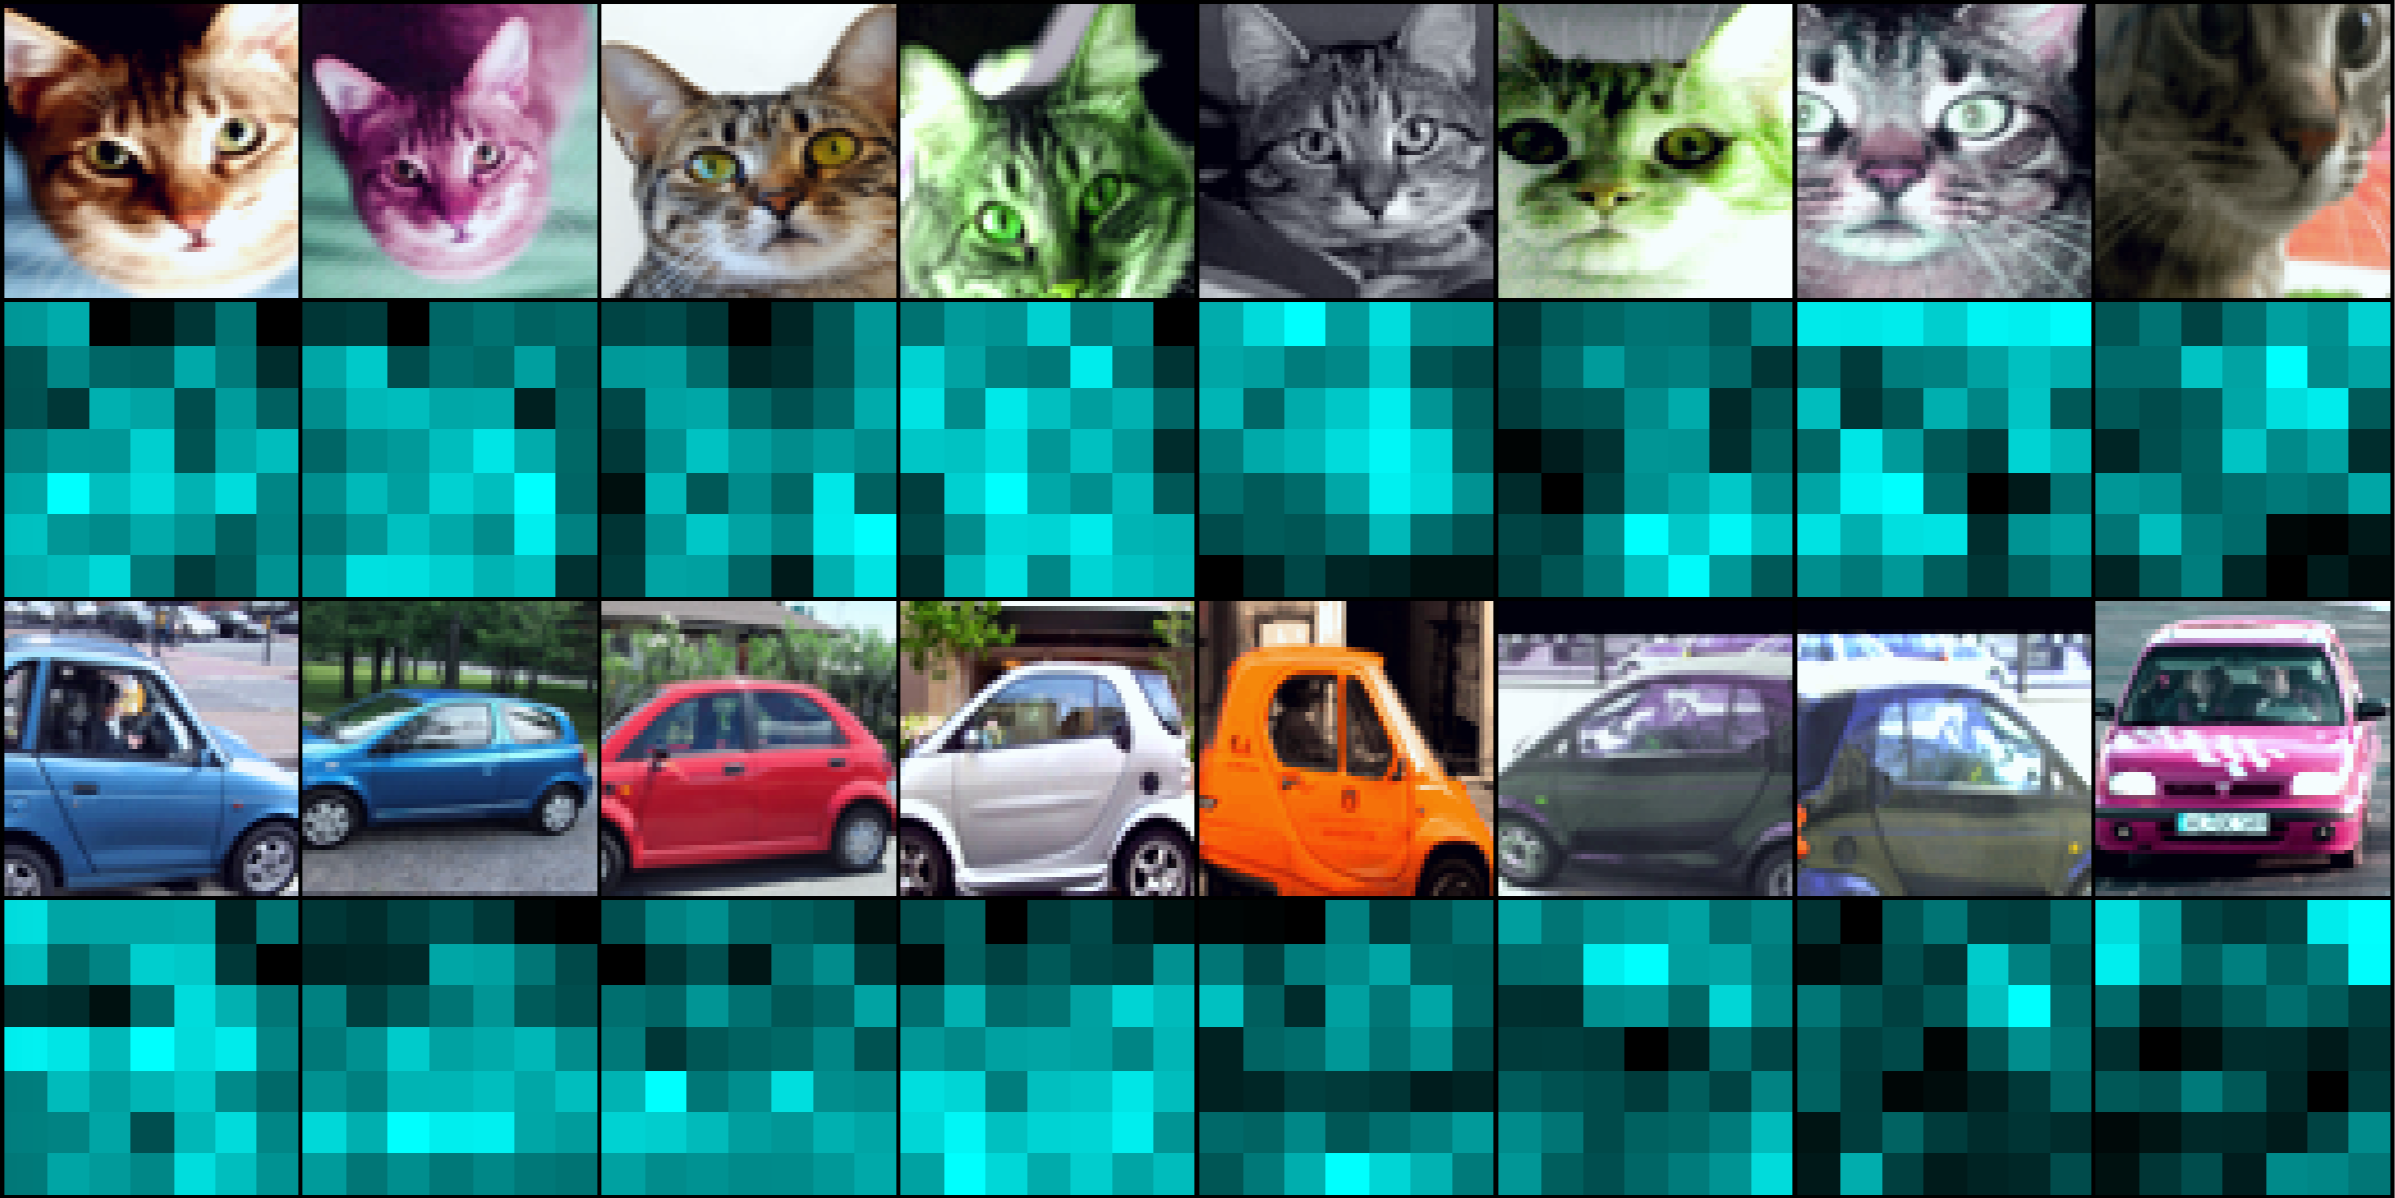}
    \caption{Successful retrieval on STL10. Format matches Fig.~\ref{fig:model_failure}.}
    \label{fig:stl10_success}
\end{figure}
